# Supplementary material for: Deep Learning Assisted Data Inspection for Radio Astronomy
Source: arXiv:2005.13373 source file (2020-05-27)
Supplement: Supplementary file 1 [file Appendix.tex]

\appendix

\section{Some extra material}

If you want to present additional material which would interrupt the flow of the main paper,
it can be placed in an Appendix which appears after the list of references.
